# Supplementary material for: Cue-CoT: Chain-of-thought Prompting for Responding to In-depth Dialogue Questions with LLMs
Source: arXiv:2305.11792 source file (2023-10-15)
Supplement: Supplementary file 1 [file case_sta_pro_std.tex]

\begin{table*}[h]
    \centering
    \begin{adjustbox}{max width=\textwidth}
    \begin{tabular}{l|l}
    \toprule
    \multicolumn{2}{c}{\textbf{Question}} \\
    \hline

    \multicolumn{2}{l}{If I had a gun right now I would kill myself. I really wish I owned a gun. I just want my life to end in a quick and painless manner. done deciding if I want live or not} \\
    \multicolumn{2}{l}{I know for a fact even if it hurts my family. I have any friends to hurt with my death so good I guess. tired of the empty feeling I wake up with every morning and the} \\
    \multicolumn{2}{l}{hard work I do just to stay alive when I even want to live. so fucking tired of it all.} \\

    % \multicolumn{2}{l}{If I had a gun right now I would kill myself. I really wish I owned a gun.} \\
    % \multicolumn{2}{l}{I just want my life to end in a quick and painless manner. done deciding if I want to live or not I know for a fact even if it hurts my family.}
    %  \\
    % \multicolumn{2}{l}{I have any friends to hurt with my death so good I guess. tired of the empty feeling I wake up with every morning and the hard work }
    %  \\
    %  \multicolumn{2}{l}{I do just to stay alive when I even want to live. so fucking tired of it all.}
    \hline
    \hline

    \multicolumn{2}{c}{\textbf{Standard Prompting}}  \\
    \hline
    \textbf{Input-1} & This is the user's question:\colorbox{yellow}{[Question]}\\
    & Please generate a response based on the user's question using first-person wording.\\
    \hdashline

     \textbf{Response-1} & I am sorry to hear that you are going through such a difficult time. It sounds like you are feeling very overwhelmed and hopeless right now. However, \\
     & I want you to know that there is help available to you. Please reach out to a trusted friend or family member, or consider contacting a professional \\
     & for support. Suicide is not the answer, and there are people who care about you and want to help you through this. Please take care of yourself and \\
     & know that there is hope for a better future. \\
     
    % \textbf{Response-1} & I am sorry to hear that you are going through such a difficult time. It sounds like you are feeling very overwhelmed and hopeless right now. \\
    % & However, I want you to know that there is help available to you. Please reach out to a trusted friend or family member, \\
    % & or consider contacting a professional for support. Suicide is not the answer, and there are people who care about you and want to help you through this. \\
    % & Please take care of yourself and know that there is hope for a better future.\\
    
    \hline
    \hline
    
    \multicolumn{2}{c}{\textbf{StatusCoT}}  \\
    \hline
    \textbf{Input-1} & This is the user's question:\colorbox{yellow}{[Question]}\\
    & Please first output a single line containing user status such as the user's personality traits, and psychological and emotional states exhibited in \\
    & the question. In the subsequent line, please generate a response based on the user's status and the user's question using first-person wording. \\
    
    % & Please first output a single line containing user status such as the user's personality traits, and psychological and \\
    % & emotional states exhibited in the question. In the subsequent line, please generate \\
    % & a response based on the user's status and the user's question using first-person wording.\\

    \hdashline
    \textbf{Response-1} & 
    \colorbox{blue!20}{Based on the user's question, it seems like they are experiencing severe depression and hopelessness. They may be struggling with suicidal ideation} \\ 
    & \colorbox{blue!20}{and feeling a sense of emptiness in their life.} \\
    
    % Based on the user's question, it seems like they are experiencing severe depression and hopelessness. \\
    % & They may be struggling with suicidal ideation and feeling a sense of emptiness in their life.\\

    % & Response:  \\
    % & I am sorry to hear that you are feeling this way. Please know that there is help available and you do not have to go through this alone. \\
    % & It's important to reach out to a mental health professional or a crisis hotline for support. Your life is valuable \\
    % & and there are people who care about you, even if it may not feel like it right now. Please take care of yourself and seek help.\\
    & \colorbox{green!20}{I am sorry to hear that you are feeling this way. Please know that there is help available and you do not have to go through this alone. It's} \\
    & \colorbox{green!20}{important to reach out to a mental health professional or a crisis hotline for support. Your life is valuable and there are people who care about} \\
    & \colorbox{green!20}{you, even if it may not feel like it right now. Please take care of yourself and seek help.} \\
    
    \hline
    \hline
    \multicolumn{2}{c}{\textbf{ProcessCoT}}  \\
    \hline
    \textbf{Input-1} & This is the user's question:\colorbox{yellow}{[Question]}\\
    & Based on the user's question, please try to infer his or her personality traits, psychological state, and emotional state as much as possible. Also, make \\
    & sure your answers are concise and easy to understand.\\

    \hdashline
    \textbf{Response-1} &  \colorbox{blue!20}{Personality traits: The user seems to have a negative outlook on life and may be prone to pessimism and self-pity.} \\
    & \colorbox{blue!20}{Psychological state: The user may be feeling overwhelmed and helpless, leading to feelings of depression and anxiety.} \\
    & \colorbox{blue!20}{Emotional state: The user is likely feeling frustrated, disappointed, and unhappy with the way their year has started.} \\
    & \colorbox{blue!20}{They may also feel isolated and unsupported due to their mention of being alone on New Year's.} \\
    \hline
    
    \textbf{Input-2} & This is user's status. \\
    & \colorbox{blue!20}{Personality traits: The user seems to have a negative outlook on life and may be prone to pessimism and self-pity.} \\
    & \colorbox{blue!20}{Psychological state: The user may be feeling overwhelmed and helpless, leading to feelings of depression and anxiety.} \\
    & \colorbox{blue!20}{Emotional state: The user is likely feeling frustrated, disappointed, and unhappy with the way their year has started.} \\
    & \colorbox{blue!20}{They may also feel isolated and unsupported due to their mention of being alone on New Year's.} \\
    
    & This is user's question:\colorbox{yellow}{[Question]}\\
    & Please generate a response based on the user's question and status using first-person wording briefly. \\
    \hdashline
    \textbf{Response-2} &  

    \colorbox{green!20}{I am deeply concerned about your well-being and safety after reading your statement. It sounds like you are experiencing intense emotional pain and} \\
    & \colorbox{green!20}{may be struggling with depression or suicidal thoughts. Please know that you are not alone and there are people who care about you and want to help.} \\
    & \colorbox{green!20}{It is important to seek immediate help from a mental health professional or a crisis hotline. Your life is valuable and you deserve to receive} \\
    & \colorbox{green!20}{support and care.} \\

    % I am deeply concerned about your well-being and safety after reading your statement. It sounds like you are experiencing \\
    % & intense emotional pain and may be struggling with depression or suicidal thoughts. Please know that you are not alone\\
    % & and there are people who care about you and want to help. It is important to seek immediate help from a \\
    % & mental health professional or a crisis hotline. Your life is valuable and you deserve to receive support and care. \\
    \bottomrule
    \end{tabular}
    \end{adjustbox}
    \caption{Demostrations of our three methods on \textbf{EMH} (\textbf{Not cherry-picking}). We highlight the intermediate reasoning results in \colorbox{blue!20}{blue} and response in \colorbox{green!20}{green}.}
    \label{tab:case_study}
\end{table*}
