# Supplementary material for: Cue-CoT: Chain-of-thought Prompting for Responding to In-depth Dialogue Questions with LLMs
Source: arXiv:2305.11792 source file (2023-10-15)
Supplement: Supplementary file 2 [file d4_example.tex]

\clearpage
\begin{CJK*}{UTF8}{gbsn}
\large
\begin{table*}[h]
    \centering
    \begin{adjustbox}{max width=\textwidth}
    \begin{tabular}{l|l}
    \toprule
    \multirow{2}{*}{\textbf{Dialogue Context}} & 用户: 您好我最近压力有点大 \\
    & \small{User: Hello, I am a little stressed recently} \\
    & 系统: 您好，在的 最近压力比较大吗？ 是哪方面的呢？工作生活？ \\
    & \small{System: Hello, Where is it from? working or life?} \\
    & 用户: 工作和家庭方面都有吧 \\
    & \small{User: Both} \\
    & 系统: 能具体讲讲吗？ 最近工作和家庭都遇到了哪些问题呢？ \\
    & \small{System: Can you talk about it more? What problems have you encountered at work and at home recently?}\\
    & 用户: 工作上我是中学老师带毕业班班主任，学生们都很难管理 \\
    & \small{User: I am a middle school teacher leading the class teacher of the graduating class, and the students are very difficult} \\
    & \small{to manage.} \\
    & 系统: 会影响到您的情绪吗？ \\
    & \small{System: Does it affect your mood?} \\
    & 用户: 会的 \\
    & \small{User: Yes!} \\
    & 系统: 比如会出现闷闷不乐、不开心？或者觉得自己能力下降？ 会自责，觉得都是自己不行？\\
    & \small{System: For example, do you feel depressed or unhappy? Or feel that your ability has declined? Would you blame yourself,} \\
    & \small{thinking that it was all your fault?} \\
    & 用户: 一方面是出于对学生的关心吧，看着他们明明都有光明的未来，但不能把握当下 另一方 \\
    & 面也是自己年纪稍微大了，感觉有点跟不上时代了 比不过那些年轻老师了 \\
    & \small{User: On the one hand, it’s because I care about the students. I see that they have a bright future, but they can’t grasp} \\
    & \small{the present moment. On the other hand, I’m a little older, and I feel a little behind the times. I can’t compare to those} \\
    & \small{young teachers.} \\
    & 系统: 嗯嗯，这个确实很头疼的，您毕竟是过来人，不想放弃每一个学生 \\
    & \small{System: Hmm, this is really tricky. After all, you are an experienced person, and you don’t want to give up every student.} \\
    & 用户: 对，他们比我的孩子还小一点 \\
    & \small{User: yes, they are a little younger than my kids} \\
    & 系统: 但是您教学经验丰富啊，这些经验不是年轻老师能有的 可能在精力体力上会稍稍差些 \\
    & 但您也有自己的长处啊\\
    & \small{System: But you have rich teaching experience, which is not something young teachers can have. You may be a little weaker} \\
    & \small{in energy and physical strength, but you also have your own strengths.} \\
    & 用户: 毕业班的老师体力精力要求确实高 我在考虑之后不带毕业班了 \\
    & \small{User: The teachers in the graduating class are really demanding physically and mentally. I am considering not taking the} \\
    & \small{graduating class after.} \\
    \hline
    \hline
    \textsc{Ground Truth} & 是的，其实这个问题也简单，您要是真的觉得自己目前的状态稍差，那您就接受当下的自 \\
    & 己，不带毕业班还可以去带别的班级，您的力量在哪里都会体现的 \\
    & \small{User: Yes, in fact, this question is also simple. If you really feel that your current state is slightly worse, then you} \\
    & \small{accept the current self, and you can take other classes without taking the graduation class. Your strength will be} \\
    & \small{reflected everywhere.} \\
    \hline
    \textsc{belle-llama-7b-2m} & 确实，别担心，您还有时间去做其他的事情。不要因为一个小插曲影响到您的整个生活。\\
    & 您可以试着找一些放松的方式，比如听音乐、散步、运动等等，来缓解您的压力。\\
    & \small{Yes, don't worry, you still have time for other things. Don't let a small episode affect your whole life. You} \\
    & \small{can try to find some relaxing ways, such as listening to music, walking, exercising, etc., to relieve your stress.} \\
    \hline
    \textsc{chatglm-6b} & 您好，我是您的系统。您最近压力比较大，能和我分享一下具体的情况吗？我可以帮助您 \\
    & 找到一些解决方案。 \\
    & \small{Hello, I am your system. You have been under a lot of pressure recently, can you share with me the specific} \\
    & \small{situation? I can help you find some solutions.} \\
    \hline
    \textsc{chatgpt} & 您拥有丰富的教学经验和知识，这些是年轻老师所没有的。虽然在精力和体力上可能有些 \\
    & 不足，但您也有自己的长处和特点。或许您可以考虑调整自己的教学方式和方法，以更好 \\
    & 地应对当前的教学环境。 \\
    & \small{You have a wealth of teaching experience and knowledge that young teachers do not have. Although you may be somewhat} \\
    & \small{lacking in energy and physical strength, you also have your own strengths and characteristics. Perhaps you could consider} \\
    & \small{adapting your teaching style and approach to better respond to your current teaching environment.} \\
    \hline
    \bottomrule
    \end{tabular}
    \end{adjustbox}
    \caption{A dialogue example from \textbf{D4} dataset using standard prompting (\textbf{Not cherry-picking}).}
    \label{tab:d4_example}
\end{table*}
\end{CJK*}
