# Supplementary material for: Cue-CoT: Chain-of-thought Prompting for Responding to In-depth Dialogue Questions with LLMs
Source: arXiv:2305.11792 source file (2023-10-15)
Supplement: Supplementary file 3 [file ed_example.tex]

\begin{table*}[h]
    \centering
    \begin{adjustbox}{max width=\textwidth}
    \begin{tabular}{l|l}
    \toprule
    \hline
    \textbf{Dialogue Context} & User: One morning my mother came to my house to pick my daughter up for school and told me she saw my daughter's cat on \\
    & the road and he had been hit. I had to tell my daughter about the loss of her beloved pet. \\
    & System: Oh no that is terrible!  How did your daughter take it? \\
    & User: She was around 11, so she took it very hard. I went ahead and let her stay home from school, as I knew she wouldn't \\
    & do well that day. \\
    \hline
    \hline
    \textsc{ground truth} & Oh poor thing.  I hope she is doing better now.  Losing a pet is extremely hard! \\    
    \hline
    % \textsc{flan-t5-xxl} & How did she feel about it? Did she feel she deserved to stay home? \\
    % \hline
    \textsc{alpaca-7b} & I'm so sorry to hear that. I can't imagine how hard that must have been for your daughter. \\
    \hline
    \textsc{vicuna-7b-v1.1} & Oh no, I can only imagine how difficult that must have been for your daughter. It's never easy to lose a beloved pet, and \\
    & it sounds like you were there to support her during a difficult time. It's understandable that you let her stay home from \\
    & school, as it can be hard to focus on anything else when you're grieving. I'm sorry for your loss and for your \\
    & daughter's. \\
    \hline
    \textsc{chatgpt} & I'm so sorry to hear that your daughter's cat passed away. Losing a pet can be incredibly difficult, especially for a \\
    & young child. It was thoughtful of you to let her stay home from school to process her emotions. Is there anything else I \\
    & can do to assist you during this difficult time?\\
    \bottomrule
    \end{tabular}
    \end{adjustbox}
    \caption{A dialogue example from \textbf{ED} dataset using standard prompting (\textbf{Not cherry-picking}).}
    \label{tab:ed_example}
\end{table*}
