# Supplementary material for: Cue-CoT: Chain-of-thought Prompting for Responding to In-depth Dialogue Questions with LLMs
Source: arXiv:2305.11792 source file (2023-10-15)
Supplement: Supplementary file 4 [file emh_example.tex]

\begin{table*}[h]
    \centering
    \begin{adjustbox}{max width=\textwidth}
    \begin{tabular}{l|l}
    \toprule
    \hline
    \textbf{Question} & Feeling dead inside. For the last 1-2 weeks feeling nothing inside, like most of the other people, dont know what to do. \\
    & Thoughts in the middle of the night well, i might die, i dont have what to live for. Literally void of nothing, black \\
    & space. \\
    \hline
    \hline
    \textsc{ground truth} & As someone who's felt the same, what do you have? And I'm speaking objectively, because I typically don't want to admit \\
    & that I have what I need when I feel as you do. Not that I'm saying that you do have a lot, but your post doesn't \\
    & necessarily shed a lot of light on what's going on. It's easy, or it has been for me, at least, to say that I don't know \\
    & what to live for, in the past. Somebody out there cares, man/woman, small or large. I don't know what your situation is, \\
    & by your post, but feel free to message me if you want. \\    
    \hline
    % \textsc{flan-t5-xxl} & Feeling dead inside means feeling like there is nothing in your life. You don’t have a sense of purpose and you don’t \\
    % & feel like you have a reason to live. You have no one to turn to or talk to. Depression is a serious condition that \\
    % & affects many people. Depression causes thoughts about death, suicidal thoughts, feelings of worthlessness, and feelings \\
    % & of hopelessness. Depression can last for a few weeks to a few months. Depression is caused by a chemical imbalance in the \\
    % & brain. Depression can be caused by a physical illness, such as a heart attack or cancer. Depression can also be caused by \\
    % & an emotional problem, such as a break up. There are many ways to treat depression, such as talking to a therapist and \\
    % & taking medication.\\
    % \hline
    \textsc{alpaca-7b} & I'm feeling really empty inside. It's like I'm not connecting with anything, even the people I care about. I feel like \\
    & I'm just existing, but not really living. It's like a void of nothingness inside of me that's making me feel scared and \\
    & alone. I'm not sure what to do to feel alive again.\\
    \hline
    \textsc{vicuna-7b-v1.1} & I'm sorry to hear that you're feeling this way. It can be really tough to feel like you're not living up to your \\
    & potential or like you don't have a purpose in life. It's important to remember that you are not alone in these feelings, \\
    & and that many people have gone through similar experiences. One thing that might help is to try to identify what is \\
    & causing you to feel this way. Is there something specific that is bothering you, or do you feel generally unfulfilled in \\
    & your life? Sometimes it can be helpful to talk to a therapist or trusted friend about your feelings, as they may be able \\
    & to offer you some perspective and support. It's also important to take care of yourself during these difficult times. \\
    & This might mean setting aside time to do things that bring you joy, such as hanging out with friends or pursuing a hobby. \\
    & It's also important to try to get enough sleep and to eat healthy foods, as these can impact how you feel. Remember that \\
    & things may not change overnight, but by taking steps to care for yourself and seeking support when you need it, you can \\
    & start to feel better over time.\\
    \hline
    \textsc{chatgpt} & I'm sorry to hear that you're feeling that way. It sounds like you're experiencing a sense of emptiness and hopelessness. \\
    & Have you considered reaching out to a mental health professional for support? They can help you work through these \\
    & thoughts and feelings and find ways to cope with them. It's important to remember that you're not alone and there is help \\
    & available. You deserve to feel happy and fulfilled in life, and with the right support, you can work towards achieving \\
    & that. \\
    \bottomrule
    \end{tabular}
    \end{adjustbox}
    \caption{A dialogue example from \textbf{EMH} dataset using standard prompting (\textbf{Not cherry-picking}).}
    \label{tab:emh_example}
\end{table*}
