# Supplementary material for: Cue-CoT: Chain-of-thought Prompting for Responding to In-depth Dialogue Questions with LLMs
Source: arXiv:2305.11792 source file (2023-10-15)
Supplement: Supplementary file 5 [file psyqa_example.tex]

\begin{CJK*}{UTF8}{gbsn}
\large
\begin{table*}[h]
    \centering
    \begin{adjustbox}{max width=\textwidth}
    \begin{tabular}{l|l}
    \toprule
    \hline
    \textbf{Question} & 成绩不合格久久不能恢复，我怎么那么容易被挫折打倒？\\
    & \small{I can't recover from failing grades for a long time. Why am I so easily defeated by setbacks?} \\
    \hline
    \textbf{Description} & 得知成绩没合格，为什么我久久不能恢复过来，我知道我复习的时间少，可能是这次失败 \\
    & 的原因。但是我心里依然难受，自己真的那么容易被打倒吗？我想不通？为啥会难受？我 \\
    & 该怎么办？ \\
    & \small{Knowing that the grades failed, why I couldn't recover for a long time, I know that I have less time to review, which may} \\
    & \small{be the reason for this failure. But I still feel uncomfortable in my heart. Is it really so easy to be defeated? I can't} \\
    & \small{figure it out? Why is it uncomfortable? what do I do?} \\
    \hline
    \hline
    \textsc{Ground Truth} &  楼主你好得知自己的成绩不合格，难受，虽然知道这个事情的主要原因是复习的少，但是 \\
    & 还是忍不住的难受。楼主其实已经知道了原因，却还是很难受，那么楼主就可以去探究为 \\
    & 什么难受？是因为自己没有看书么？是因为这次的题太简单？还是觉得自己没过会受到环 \\
    & 境的影响？你需要把这里的关系理清楚，找到自己难受的根源，然后对症下药。楼主可以 \\
    & 去听听音乐，做点运动，或者旅游放松自己的心情，其实楼主不必把这种事情放的太重， \\
    & 不合格又如何，会受罚？会挨骂？还是会被嘲笑？即便如此那又如何。我的人生我做主， \\
    & 何必在乎那么多看法。找到你人生的目标，楼主说了看书少，也什么会看书少，是因为没 \\
    & 有动力还是没有兴趣，如果做一件喜欢的事情你会不会也是如此？你要问问自己，了解自 \\
    & 己究竟想要什么，没有目标就不会用心对一件事情，有方向能坚持会事半功倍，加油。\\
    & \small{Hello, it seems that you have received news that your grades are not satisfactory, and you're feeling upset about} \\
    & \small{it. Although you understand that the main reason for this outcome is due to insufficient studying, you still can't help} \\
    & \small{feeling distressed. It may be helpful to investigate why you're feeling this way. Is it because you didn't study enough?} \\
    & \small{Are the questions too easy, making you feel like you didn't accomplish anything? Or are you worried about how your} \\
    & \small{surroundings will perceive you if you don't pass? You need to clarify these relationships, identify the root cause of} \\
    & \small{your distress, and take appropriate action. You could try listening to music, doing some exercise, or traveling to ease} \\
    & \small{your mind. In reality, you don't need to weigh this situation too heavily. Even if you didn't pass, will you be punished,} \\
    & \small{scolded, or ridiculed? So what if you do? You are the master of your own life, and you don't need to care about what} \\
    & \small{others think. Find your life goals. You mentioned that you studied less. Is it due to a lack of motivation or interest?} \\
    & \small{Would you behave similarly if you were doing something you enjoyed? Ask yourself these questions, understand what you} \\
    & \small{want, and set goals for yourself. Without direction, you won't be able to commit yourself fully to any task, but with a} \\
    & \small{clear direction, you can accomplish more with less effort. Keep going!} \\
    \hline
    \textsc{belle-llama-7b-2m} & 我曾经也遇到过这样的困境，我知道我的学习时间可能不够，但是我从来没有放弃过。我 \\
    & 觉得我需要做的是重新评估我的学习计划，找出我的问题并寻找解决方案。我可能需要更 \\
    & 多的时间来复习，或者找出更好的学习方法。我也需要更多的鼓励和支持，来保持积极的 \\
    & 心态和勇气。我相信只要我坚持努力，我一定能够恢复和进步。\\
    & \small{I have also encountered such a dilemma. I know that my study time may not be enough, but I never give up. I feel like} \\
    & \small{what I need to do is re-evaluate my study plan, identify my problems and look for solutions. I might need more time to} \\
    & \small{review, or figure out a better way to study. I also need more encouragement and support to stay positive and courageous.} \\
    & \small{I believe that as long as I keep working hard, I will be able to recover and improve.} \\
    \hline
    \textsc{chatglm-6b} & 得知成绩不合格，久久不能恢复过来，感觉自己很容易被挫折打倒，可能是因为自己过于 \\
    & 在意这次失败。当我得知成绩不合格时，我的心情非常低落，感觉自己付出了很多努力，\\
    & 但最终却失败了。这种失落感和挫败感很容易让我失去信心和勇气。我也明白复习的时间 \\
    & 少可能是这次失败的原因之一，但我认为这只是这次失败的主要原因之一。我可能需要更 \\
    & 多的时间和努力来提高自己的能力和技能。当我遇到挫折时，我会试着找出原因和解决方 \\
    & 法。我知道我需要更加努力地学习，制定更合理的学习计划，并安排更多的时间来复习和 \\
    & 准备考试。我也会和朋友和家人交流，寻求他们的鼓励和支持。最后，我想强调的是，不 \\
    & 要轻易放弃。即使我遇到挫折，我也要相信自己能够克服难关，取得成功。我会继续努力, \\
    & 不断提高自己的能力和素质，为实现自己的梦想而不断努力。\\
    & \small{When I learned that my grades were unqualified, I couldn’t recover for a long time. I felt that I was easily overwhelmed} \\
    & \small{by setbacks. Maybe it was because I cared too much about this failure. When I was informed that I had failed my grades, I} \\
    & \small{was very depressed and felt like I had put in a lot of effort and failed in the end. This sense of loss and frustration} \\
    & \small{can easily make me lose confidence and courage. I also understand that the lack of review time may be one of the reasons} \\
    & \small{for this failure, but I think this is only one of the main reasons for this failure. I may need more time and effort to} \\
    & \small{improve my abilities and skills. When I encounter setbacks, I try to find out the reasons and solutions. I know that I} \\
    & \small{need to study harder, make a more reasonable study plan, and arrange more time to review and prepare for the exam. I also} \\
    & \small{talk to friends and family and seek their encouragement and support. Finally, I want to emphasize that don't give up} \\
    & \small{easily. Even when I encounter setbacks, I have to believe that I can overcome them and succeed. I will continue to work} \\
    & \small{hard, continuously improve my ability and quality, and continue to work hard to realize my dreams.} \\
    \hline
    \bottomrule
    \end{tabular}
    \end{adjustbox}
    \caption{A dialogue example from \textbf{PsyQA} dataset using standard prompting (\textbf{Not cherry-picking}).}
    \label{tab:psyqa_example}
\end{table*}
\end{CJK*}
