# Supplementary material for: Cue-CoT: Chain-of-thought Prompting for Responding to In-depth Dialogue Questions with LLMs
Source: arXiv:2305.11792 source file (2023-10-15)
Supplement: Supplementary file 6 [file psyqa_example_extend.tex]

\begin{CJK*}{UTF8}{gbsn}
\large
\begin{table*}[h]
    \centering
    \begin{adjustbox}{max width=\textwidth}
    \begin{tabular}{l|l}
    \toprule
    \hline
    \textbf{Question} & 成绩不合格久久不能恢复，我怎么那么容易被挫折打倒？\\
    & \small{I can't recover from failing grades for a long time. Why am I so easily defeated by setbacks?} \\
    \hline
    \textbf{Description} & 得知成绩没合格，为什么我久久不能恢复过来，我知道我复习的时间少，可能是这次失败 \\
    & 的原因。但是我心里依然难受，自己真的那么容易被打倒吗？我想不通？为啥会难受？我 \\
    & 该怎么办？ \\
    & \small{Knowing that the grades failed, why I couldn't recover for a long time, I know that I have less time to review, which may} \\
    & \small{be the reason for this failure. But I still feel uncomfortable in my heart. Is it really so easy to be defeated? I can't} \\
    & \small{figure it out? Why is it uncomfortable? what do I do?} \\
    \hline
    \hline
    \textsc{chatgpt} & 我能理解你的感受，得知成绩不合格是一件非常令人失落的事情。虽然你知道自己复习的 \\
    & 时间不够，但是心里仍然很难受，这是很正常的反应。我们都会有挫折的时候，但是如何 \\
    & 面对挫折才是最重要的。你可以先接受当前的不足，然后制定一个新的计划，更加有针对 \\
    & 性地复习，充分利用时间和资源，为下次考试做好准备。此外，你也可以寻求一些心理支 \\
    & 持和帮助，和身边的人聊聊，或者找心理咨询师倾诉自己的感受。最重要的是，不要因为 \\
    & 一次失败而放弃，要坚持努力，相信自己能够克服困难，迎接下一个挑战。 \\
    & \small{I can understand how you feel, it is very disheartening to learn that you failed your grades. Although you know that you} \\
    & \small{don't have enough time to review, you still feel uncomfortable. This is a normal reaction. We all have setbacks, but how} \\
    & \small{to deal with setbacks is the most important thing. You can accept the current deficiencies first, then make a new plan,} \\
    & \small{review more targetedly, make full use of time and resources, and prepare for the next exam. In addition, you can also} \\
    & \small{seek some psychological support and help, talk to people around you, or find a counselor to talk about your feelings. The} \\
    & \small{most important thing is not to give up because of one failure, but to keep working hard and believe that you can overcome} \\
    & \small{difficulties and meet the next challenge.} \\
    \hline
    \bottomrule
    \end{tabular}
    \end{adjustbox}
    \caption{A dialogue example from \textbf{PsyQA} dataset using standard prompting (\textbf{Not cherry-picking}).}
    \label{tab:psyqa_example_extend}
\end{table*}
\end{CJK*}
