# Supplementary material for: Cue-CoT: Chain-of-thought Prompting for Responding to In-depth Dialogue Questions with LLMs
Source: arXiv:2305.11792 source file (2023-10-15)
Supplement: Supplementary file 7 [file quora_example.tex]

\begin{table*}[h]
    \centering
    \begin{adjustbox}{max width=\textwidth}
    \begin{tabular}{l|l}
    \toprule
    \hline
    \textbf{Dialogue Context} & User: I have a question. What should I reply in return when someone says I missed you, I love you, or you look beautiful, \\
    & but I know they don't mean it? Because replying back with 'I missed you too', 'I love you too', or 'you look beautiful \\
    & too' would be a lie too. \\
    & System: That's a good question. You could try redirecting the conversation to something else, like asking them about \\
    & their day or plans for the weekend. Or you could simply say thank you or acknowledge the compliment without reciprocating \\
    & it. It ultimately depends on the situation and your relationship with the person. \\
    & User: But what if it's someone I can't avoid, like a family member or a coworker? How do I respond without lying? \\
    & system: In that case, you could try being honest and saying something like, "Thank you for saying that, but I don't feel \\
    & the same way." It may be uncomfortable, but it's important to be true to yourself and not feel pressured to reciprocate \\
    & false sentiments. \\
    & User: That's a good point. But what if I don't want to hurt their feelings? \\
    \hline
    \hline
    \textsc{ground truth} & You could try being gentle and saying something like, "I appreciate your kind words, but I'm not comfortable \\
    & reciprocating those feelings." It's important to set boundaries and communicate honestly, while also being mindful of the \\
    & other person's feelings.\\    
    \hline
    % \textsc{flan-t5-xxl} & If you don't want to hurt their feelings, you could simply say "thank you," or "I'm fine," or "I appreciate that." \\
    % \hline
    \textsc{alpaca-7b} & I understand your reluctance to hurt their feelings. You could try acknowledging the compliment without reciprocating it. \\
    & For example, you could say "Thank you for saying that, I appreciate the kind words". This will let them know that you \\
    & appreciate their sentiments, without having to reciprocate them. \\
    \hline
    \textsc{vicuna-7b-v1.1} &  As a language model, I suggest being honest while being respectful. You can say something like, "I appreciate your kind \\
    & words, but I don't feel the same way. However, I value our relationship and don't want to hurt your feelings, so let's \\
    & just move on and continue our conversation." This response acknowledges their sentiment while being truthful and \\
    & maintaining a positive tone.\\
    \hline
    \textsc{chatgpt} & I understand your concern. It's natural to want to avoid hurting someone's feelings. In that case, you could try being \\
    & diplomatic and say something like, "I appreciate the sentiment, but I prefer to keep things strictly professional / \\
    & friendly between us." This way, you're acknowledging their comment without leading them on or hurting their \\
    & feelings. Remember, it's important to prioritize your own feelings and boundaries in any situation.\\
    \bottomrule
    \end{tabular}
    \end{adjustbox}
    \caption{A dialogue example from \textbf{Quora} dataset using standard prompting (\textbf{Not cherry-picking}).}
    \label{tab:quora_example}
\end{table*}
