# Supplementary material for: Cue-CoT: Chain-of-thought Prompting for Responding to In-depth Dialogue Questions with LLMs
Source: arXiv:2305.11792 source file (2023-10-15)
Supplement: Supplementary file 8 [file zhihu_example.tex]

\begin{CJK*}{UTF8}{gbsn}
\large
\begin{table*}[h]
    \centering
    \begin{adjustbox}{max width=\textwidth}
    \begin{tabular}{l|l}
    \toprule
    \hline
    \textbf{Dialogue Context} & 用户: 考研失利等于人生失败吗？\\
    & \small{User: Is failure in the postgraduate entrance examination equal to failure in life?} \\
    & 系统: 不是，考研失利不等于人生失败，考研只是一次学习挑战，考研失败并不意味着\\
    & 自己的人生就结束了，可以从失败中汲取教训，努力改变，去实现自己的人生目标。\\
    & \small{System: No, failing the postgraduate entrance examination does not mean failure in life. It is just a learning challenge.} \\
    & \small{Failure in the postgraduate entrance examination does not mean that your life is over. You can learn from failures and} \\
    & \small{work hard to change to achieve your life goals.} \\
    & 用户: 你是怎么想的？ \\ 
    & \small{User: what do you think?} \\
    & 系统: 我认为要从失败中吸取经验教训，让自己学会从失败中变得更加强大。勇敢地去 \\ 
    & 挑战，尝试新的事物，不断的去实现自己的梦想。\\
    & \small{System: I think it is necessary to learn from failures and let yourself learn to become stronger from failures. Be brave} \\
    & \small{to challenge, try new things, and constantly realize your dreams.} \\
    & 用户: 要如何才能做到这些？\\
    & \small{User: How to achieve these?} \\
    \hline
    \hline
    \textsc{Ground Truth} & 首先要具备良好的心态，不断地保持乐观、勇敢、坚强的心态，其次要有一定的规划，明 \\
    & 确自己的目标，并且制定出合理的计划和行动方案。最后，要坚持不懈，不断努力，尽自 \\
    & 己最大的努力去实现自己的梦想。\\
    & \small{System: First of all, you must have a good attitude, and constantly maintain an optimistic, brave, and strong attitude.} \\
    & \small{Secondly, you must have a certain plan, clarify your goals, and formulate reasonable plans and action plans. Finally, we} \\
    & \small{must persevere, keep working hard, and do our best to realize our dreams.} \\
    \hline
    \textsc{belle-llama-7b-2m} & 做到这些，需要首先接受失败是成功路上的一个必经之路，不要害怕失败，而是从失败中 \\
    & 吸取经验教训，做出改变，努力实现自己的人生目标。同时，也需要不断尝试新的事物，\\
    & 勇敢地去挑战自己，相信自己的能力，让自己变得更加强大。\\
    & \small{System: To do this, you need to first accept that failure is a must on the road to success. Don't be afraid of failure,} \\
    & \small{but learn lessons from failure, make changes, and strive to achieve your life goals. At the same time, you also need to} \\
    & \small{constantly try new things, challenge yourself bravely, believe in your own abilities, and make yourself stronger.} \\
    \hline
    \textsc{chatglm-6b} & 要如何做到这些，需要先明确自己的人生目标，然后制定一个计划，并不断地去努力实现。 \\
    & 在这个过程中，需要不断学习，积累经验，并且保持积极的心态，勇于面对挑战和失败。 \\
    & 还需要有坚定的信念和毅力，去坚持不懈地追求自己的梦想。总之，要从失败中吸取经 \\
    & 验教训，让自己学会从失败中变得更加强大，并且勇敢地去挑战，尝试新的事物，不断实 \\
    & 现自己的梦想。\\
    & \small{System: To do this, you need to clarify your life goals first, then make a plan, and continue to work hard to achieve it.} \\
    & \small{In this process, it is necessary to continuously learn, accumulate experience, maintain a positive attitude, and face} \\
    & \small{challenges and failures bravely. It also requires firm belief and perseverance to persevere in pursuing your dreams. In} \\
    & \small{short, learn from failures, let yourself learn to become stronger from failures, and bravely challenge, try new things,} \\
    & \small{and constantly realize your dreams.} \\
    \hline
    \textsc{chatgpt} &  要做到这些，我认为首先要接受失败，并不要将其视为人生终点，而是将其视为人生的一 \\
    & 个阶段。然后，我们应该尝试分析失败的原因，从中吸取经验教训，并努力改变自己的不 \\
    & 足。同时，我们应该继续保持积极的心态，勇敢地去挑战新的事物，不断地学习和成长。\\
    & 最重要的是，我们应该坚持自己的梦想，为自己的人生目标而努力奋斗。无论遇到什么困 \\
    & 难和挑战，我们都应该坚定地相信自己，坚持不懈地追求自己的梦想。\\
    & \small{System: To do this, I think the first step is to accept failure, not as the end of life, but as a stage of life. Then, we} \\
    & \small{should try to analyze the reasons for the failure, draw lessons from it, and try to change our shortcomings. At the same} \\
    & \small{time, we should continue to maintain a positive attitude, bravely challenge new things, and continue to learn and grow.} \\
    & \small{Most importantly, we should stick to our dreams and work hard for our life goals. No matter what difficulties and} \\
    & \small{challenges we encounter, we should firmly believe in ourselves and pursue our dreams unremittingly.} \\
    \hline
    \bottomrule
    \end{tabular}
    \end{adjustbox}
    \caption{A dialogue example from \textbf{Zhihu} dataset using standard prompting (\textbf{Not cherry-picking}).}
    \label{tab:zhihu_example}
\end{table*}
\end{CJK*}
