# Supplementary material for: Cue-CoT: Chain-of-thought Prompting for Responding to In-depth Dialogue Questions with LLMs
Source: arXiv:2305.11792 source file (2023-10-15)
Supplement: Supplementary file 9 [file acceptness_eva_cn.tex]

\begin{table*}[!t]
    \centering
    \begin{adjustbox}{max width=\textwidth}
    \begin{tabular}{l|cc|cc|cc}
    \toprule
    \multirow{2}{*}{\textbf{Model}} & \multicolumn{2}{c|}{\textbf{Zhihu}} & \multicolumn{2}{c|}{\textbf{D4}} & \multicolumn{2}{c}{\textbf{PsyQA}}   \\
     \cline{2-7}  & \textit{ground truth} & \textit{standard} & \textit{ground truth} & \textit{standard} & \textit{ground truth} & \textit{standard} \\
    \hline
    \textsc{chatglm-6b} & 86.67 & 66.67 & 92.81 & 51.27 & 58.37 & 55.40 \\
    \textsc{belle-llama-7b-2m} & 75.71 & 60.23 & 87.23 & 72.41 & \underline{45.75} & 73.65 \\
    \textsc{ChatGPT} & \textbf{88.46} & 65.22 & \textbf{94.15} & 61.08 & \textbf{58.95} & 56.12 \\
    \bottomrule
    \end{tabular}
    \end{adjustbox}
    \caption{The win rate of responses generated by \textbf{Explicit CoT} compared with the ground truth and also response with standard prompting on three \textbf{Chinese} datasets in terms of \textbf{acceptability}.}
    \label{tab:acceptness_eva_cn}
\end{table*}
