# Supplementary material for: Cue-CoT: Chain-of-thought Prompting for Responding to In-depth Dialogue Questions with LLMs
Source: arXiv:2305.11792 source file (2023-10-15)
Supplement: Supplementary file 10 [file acceptness_eva_en.tex]

\begin{table*}[h]
    \centering
    \begin{adjustbox}{max width=\textwidth}
    \begin{tabular}{l|cc|cc|cc}
    \toprule
    \multirow{2}{*}{\textbf{Model}} & \multicolumn{2}{c|}{\textbf{Quora}} & \multicolumn{2}{c|}{\textbf{ED}} & \multicolumn{2}{c}{\textbf{EMH}}  \\
     \cline{2-7}  & \textit{ground truth} & \textit{standard} & \textit{ground truth} & \textit{standard} & \textit{ground truth} & \textit{standard} \\
    \hline
    \textsc{flan-t5-xxl} & \underline{17.10} & 52.14 & 62.02 & 55.24 & \underline{24.33} & 55.56 \\
    \textsc{alpaca-7b} & 69.15 & 78.21 & 98.79 & 86.00 & 69.54 & 86.97 \\
    \textsc{vicuna-7b-v1.1} & 90.73 & 77.89 & \textbf{99.80} & 90.71 & 97.28 & 82.93 \\
    \textsc{ChatGPT} & \textbf{96.58} & 89.09 & \textbf{99.80} & 96.79 & \textbf{97.59} & 94.93 \\
    \bottomrule
    \end{tabular}
    \end{adjustbox}
    \caption{The win rate of responses generated by \textbf{Explicit CoT} compared with the ground truth and also response with standard prompting on three \textbf{English} datasets in terms of \textbf{acceptability}.}
    \label{tab:acceptness_eva_en}
\end{table*}
