# Supplementary material for: Cue-CoT: Chain-of-thought Prompting for Responding to In-depth Dialogue Questions with LLMs
Source: arXiv:2305.11792 source file (2023-10-15)
Supplement: Supplementary file 11 [file existing_evaluation_cn.tex]

\begin{table}[!t]
    \centering
    \begin{adjustbox}{max width=0.45\textwidth}
    \begin{tabular}{l|c|cc|cc|cc}
    \toprule
    \multirow{2}{*}{\textbf{Model}} & \multirow{2}{*}{\textbf{Prompt}} & \multicolumn{2}{c|}{\textbf{Zhihu}} & \multicolumn{2}{c}{\textbf{D4}} & \multicolumn{2}{c}{\textbf{PsyQA}} \\
    \cline{3-8} & & Avg.B & F1 & Avg.B & F1 & Avg.B & F1 \\
    \hline
    \hline
    \multirow{3}{*}{\textsc{belle}} & Standard & \textbf{15.74} & \textbf{39.98} & 3.69 & 19.71 & 2.44 & 26.45 \\
    & \textit{O-Cue} & 10.43 & 30.86 & 3.32 & 17.90 & 0.96 & 18.44 \\
    & \textit{M-Cue} & 15.39 & 39.15 & \textbf{3.73} & \textbf{19.75} & \textbf{2.74} & \textbf{27.12} \\
    \hline
    \multirow{3}{*}{\textsc{chatglm}} & Standard & \textbf{10.98} & 33.23 & 3.43 & 18.79 & 7.67 & 37.64 \\
    & \textit{O-Cue}  & 12.77 & \textbf{35.55} & \textbf{4.26} & \textbf{20.86} & 1.32 & 20.22 \\
    & \textit{M-Cue} & 8.74 & 28.60 & 3.09 & 17.86 & \cellcolor{blue!30}\textbf{8.01} & \cellcolor{blue!30}\textbf{38.15} \\
    \hline
    \multirow{3}{*}{\textsc{chatgpt}}  & Standard & 14.98 & 40.35 & 4.21 & 21.09 & 6.47 & \textbf{36.86} \\
    & \textit{O-Cue}  & \cellcolor{blue!30}\textbf{16.37} & \cellcolor{blue!30}\textbf{41.40} & \cellcolor{blue!30}\textbf{5.11} & \cellcolor{blue!30}\textbf{23.20} &  2.89 & 28.70 \\
    & \textit{M-Cue} & 13.42 & 38.36 & 3.83 & 20.22 & \textbf{6.49} & 36.51\\
    \bottomrule
    \end{tabular}
    \end{adjustbox}
    \caption{The performance of existing automatic metrics such as AVG BLEU: average of BLEU-1,-2,-3,-4, and F1 under zero-shot setting on Chinese datasets. We color maximum performance.}
    \label{tab:existing_eval_cn}
\end{table}
