# Supplementary material for: Cue-CoT: Chain-of-thought Prompting for Responding to In-depth Dialogue Questions with LLMs
Source: arXiv:2305.11792 source file (2023-10-15)
Supplement: Supplementary file 12 [file existing_evaluation_en.tex]

\begin{table}[!t]
    \centering
    \begin{adjustbox}{max width=0.45\textwidth}
    \begin{tabular}{l|c|cc|cc|cc}
    \toprule
    \multirow{2}{*}{\textbf{Model}} & \multirow{2}{*}{\textbf{Prompt}} & \multicolumn{2}{c|}{\textbf{Quora}} & \multicolumn{2}{c}{\textbf{ED}} & \multicolumn{2}{c}{\textbf{EMH}} \\
    \cline{3-8} & & Avg.B & F1 & Avg.B & F1 & Avg.B & F1 \\
    \hline
    \hline
    % \multirow{3}{*}{\textsc{flan-t5-xxl}} & Standard & 23.65 & 57.51 & \cellcolor{blue!30}\textbf{32.38} & 57.24 & \textbf{1.98} & \textbf{33.91} \\
    % & \textit{O-Cue} & \textbf{26.34} & 57.05 & 29.76 & 56.00 & 0.23 & 27.10 \\
    % & \textit{M-Cue} & 23.72 & \textbf{57.52} & 31.38 & \cellcolor{blue!30}\textbf{57.40} & 0.93 & 30.14 \\
    % \hline
    \multirow{3}{*}{\textsc{alpaca}} & Standard & 52.99 & 72.53 & \textbf{25.32} & \textbf{51.96} & 6.10 & 45.45 \\
    & \textit{O-Cue} & 32.92 & 63.28 & 23.97 & 51.22 & 0.64 & 31.70 \\
    & \textit{M-Cue} & \cellcolor{blue!30}\textbf{53.16} & \cellcolor{blue!30}\textbf{73.81} & 22.73 & 48.41 & \textbf{8.49} & \textbf{49.58}  \\
    \hline
    \multirow{3}{*}{\textsc{vicuna}} & Standard & 40.50 & 66.32 & 15.60 & 36.95 & \cellcolor{blue!30}\textbf{54.87} & 74.47 \\
    & \textit{O-Cue} & \textbf{51.12} & \textbf{71.90} & \textbf{17.87} & \textbf{45.61} & 28.70 & 68.38 \\
    & \textit{M-Cue} & 37.43 & 62.35 & 13.43 & 32.59 & 46.12 & \textbf{74.72} \\
    \hline
    \multirow{3}{*}{\textsc{chatgpt}} & Standard & \textbf{51.64} & 73.44 & 15.70 & 34.37 & \textbf{42.05} & \cellcolor{blue!30}\textbf{74.85} \\
    & \textit{O-Cue} & 51.57 & \textbf{73.61} & \textbf{16.01} & \textbf{35.14} & 35.97 & 72.78 \\
    & \textit{M-Cue} & 47.48 & 70.10 & 13.77 & 30.47 & 39.88 & 74.76 \\
    \bottomrule
    \end{tabular}
    \end{adjustbox}
    \caption{The performance of existing automatic metrics such as AVG BLEU: average of BLEU-1,-2,-3,-4, and F1 under zero-shot setting on English datasets. We color maximum performance.}
    \label{tab:existing_eval_en}
    \vspace{-6mm}
\end{table}
